# Supplementary material for: Not Low-Resource Anymore: Aligner Ensembling, Batch Filtering, and New Datasets for Bengali-English Machine Translation
Source: arXiv:2009.09359 source file (2020-10-07)
Supplement: Supplementary file 1 [file supplementary.tex]

\section{Supplemental Material}
\label{sec:supplemental}
Submissions may include non-readable supplementary material used in the work and described in the paper.
Any accompanying software and/or data should include licenses and documentation of research review as appropriate.
Supplementary material may report preprocessing decisions, model parameters, and other details necessary for the replication of the experiments reported in the paper.
Seemingly small preprocessing decisions can sometimes make a large difference in performance, so it is crucial to record such decisions to precisely characterize state-of-the-art methods. 

Nonetheless, supplementary material should be supplementary (rather than central) to the paper.
\textbf{Submissions that misuse the supplementary material may be rejected without review.}
Supplementary material may include explanations or details of proofs or derivations that do not fit into the paper, lists of
features or feature templates, sample inputs and outputs for a system, pseudo-code or source code, and data.
(Source code and data should be separate uploads, rather than part of the paper).

The paper should not rely on the supplementary material: while the paper may refer to and cite the supplementary material and the supplementary material will be available to the reviewers, they will not be asked to review the supplementary material.
