# Supplementary material for: Not Low-Resource Anymore: Aligner Ensembling, Batch Filtering, and New Datasets for Bengali-English Machine Translation
Source: arXiv:2009.09359 source file (2020-10-07)
Supplement: Supplementary file 2 [file appendix.tex]

\appendix
\section{Appendices}
\label{sec:appendix}
Appendices are material that can be read, and include lemmas, formulas, proofs, and tables that are not critical to the reading and understanding of the paper. 
Appendices should be \textbf{uploaded as supplementary material} when submitting the paper for review.
Upon acceptance, the appendices come after the references, as shown here.

\paragraph{\LaTeX-specific details:}
Use {\small\verb|\appendix|} before any appendix section to switch the section numbering over to letters.
